# Supplementary material for: Follow-Your-Click: Open-domain Regional Image Animation via Short Prompts
Source: arXiv:2403.08268 source file (2024-03-13)
Supplement: Supplementary file 1 [file supp_mask_condition.tex]

\begin{figure*}[t]
  \centering
  \begin{tabular}{c@{\hspace{0.1em}}c@{\hspace{0.1em}}c@{\hspace{0.1em}}c@{\hspace{0.1em}}c@{\hspace{0.1em}}c}
  OF-G  & Output &  SAM-G & Output  \\
  % & {\small I2VGen-XL}~\cite{i2vgenxl} & {\small RegionMaker(ours)}\\
    \includegraphics[width=0.2\linewidth]{images/mask_optical.png} &
    \animategraphics[width=0.2\linewidth]{8}{gif/supp_mask/optical/frame_}{1}{16}&
     \includegraphics[width=0.2\linewidth]{images/mask_sam.png}&
     \animategraphics[width=0.2\linewidth]{8}{gif/supp_mask/sam/frame_}{1}{16}
     % % \includegraphics[width=0.14\linewidth]{gif/AZvsOthers/line3/videocrafter/011_0.jpg}&
     % \animategraphics[width=0.2\linewidth]{8}{gif/ablation_motion/OFC_16/frame_}{1}{16}
     % \\
     % \multicolumn{2}{c}{\textit{``walking, driving''}}  & \multicolumn{2}{c}{\textit{``dancing''}} &  &  \\
    \end{tabular}
    
\vspace{-0.7em}
  \caption{\textbf{The comparison between different conditional mask}. \enquote{OF-G} is the mask from optical flow-based motion mask generation and \enquote{SAM-G} .
  % \textit{Best viewed with Acrobat Reader. Click the video to play the animation clips. \textbf{Static frames are provided in supplementary materials.}}
  }
  \vspace{-0.3cm}
\label{fig:mask_different} 
\end{figure*}
% }
